# Supplementary material for: Augmenting Policy Learning with Routines Discovered from a Single Demonstration
Source: arXiv:2012.12469 source file (2021-05-02)
Supplement: Supplementary file 1 [file s2_Additional_exps.tex]

\section{Additional Ablation Study}
\subsection{Effect of Parameters in Routine Abstraction}
\label{sec:ablation_paras}
We validate the effectiveness of the parameters used in routine abstraction: the balancing factor $\lambda$, the similarity threshold $n$ and the number of routines $k$. We denote the default parameters (presented in Sec \ref{sec: hyperparameters}) as $\lambda_d$, $n_d$, and $k_d$. For each parameter, we change into different values while other parameters are set to the default values. 

As in other ablation studies in our paper, we train the routine policy via PPO on CoinRun's hard levels. The number of training levels is unbounded while we restrict a training budget of 50k episodes. We report the mean reward of the last 100 episodes. Each experiment is averaged for three seeds.

We show abstracted routine libraries for different parameters in Table \ref{tb:routine_libraries}. Note we only show routines that are not primitive actions. The qualitative results are shown in Figure \ref{Fig:ablation_paras}. We analyze the results in the following paragraphs.

\subsubsection{Balancing Factor} 
A smaller balancing factor indicates a weaker effect of the lengths of routines. When the balancing factor is very small ($\lambda=0.1 \lambda_d)$, the abstracted routines are very short such as \texttt{[RIGHT, RIGHT, RIGHT]}. These routines are ineffective because they are too short to carry enough information as skills. Besides, selecting routines mainly according to the routine length (when $\lambda=100\lambda_d$) is also ineffective because these routines are rarely used.

\subsubsection{Similarity Threshold}
Preventing adding too similar routines is also important. When $n$ is very small, there are too many similar routines in one routine library. Such routines have similar functions and would slow down exploration. On the other hand, when $n$ is very large, too many routines would be pruned. So the abstracted routines are not the ones with best scores. Therefore, a moderate $n$ leads to the best performance.

\subsubsection{Selected Number of Routines}
The number of adopted routines also influences the performance of the training process. Although selecting only one routine can increase the solved levels, abstracting a few more routines can have stronger performance. A too-large routine library would harm performance because a large action space would lead to inefficient exploration.

\subsection{Effect of Adopting the Minimal Action Space on CoinRun}
\label{Sec:minimum action space}
On CoinRun, for the sake of clear presentation, we adopt the minimal action space and remove all the predefined combos (e.g., \texttt{RIGHTDOWN}). Note that the baselines also use the minimal action space in previous experiments on CoinRun. Figure \ref{Fig:ablation_action_space} shows the training curves of routine policies based on full action space and minimum action space. Our routine abstraction and routine policy training algorithm can work even better when adopting the full action space.

\begin{figure}[t]
\vskip 0.2in
\begin{center}
\centerline{
\subfig\includegraphics[width=0.9\columnwidth]{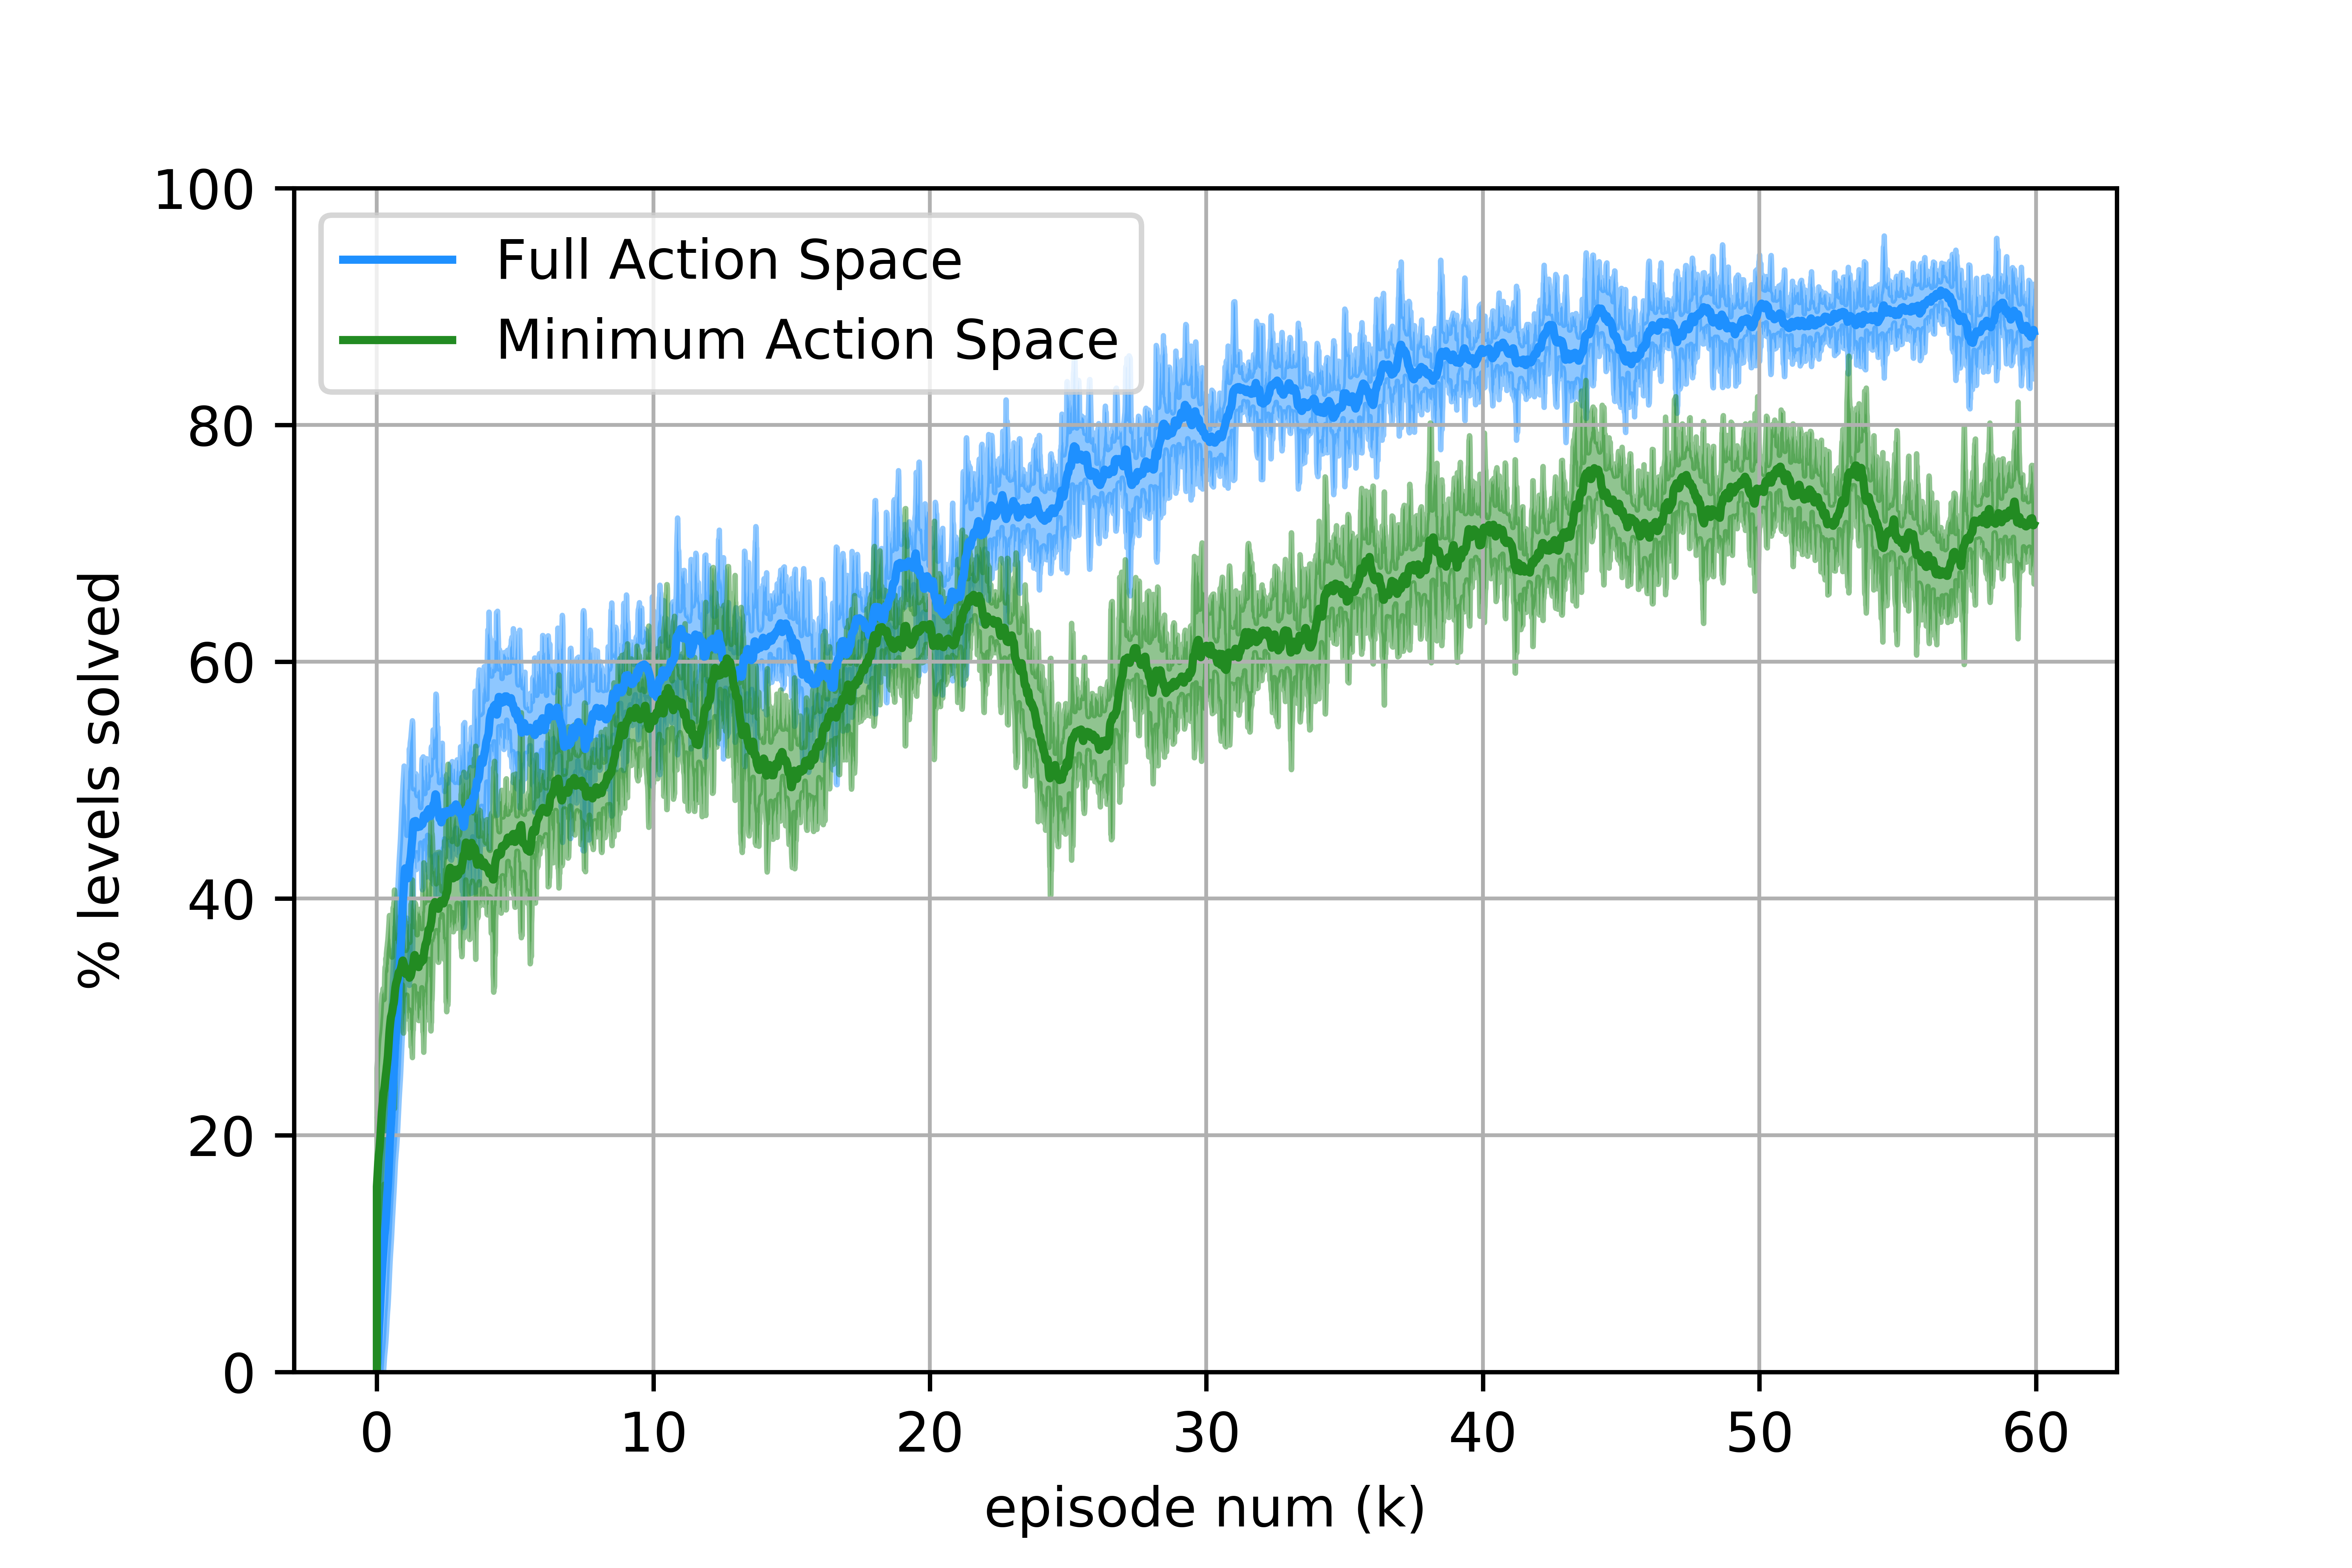}}
\caption{Compare routine policies based on full action space and minimum action space. Although training on full action space has stronger performance, for the sake of better interpretation, we adopt the minimum action space on CoinRun. Refer to Sec \ref{Sec:minimum action space} for more details.}
\label{Fig:ablation_action_space}
\end{center}
\vskip -0.2in
\end{figure}
